# Supplementary material for: Synthesizing Reactive Systems from Hyperproperties
Source: arXiv:1905.13511 source file (2019-05-31)
Supplement: Supplementary file 1 [file experiments_appendix.tex]

\section{Experiments} \label{sec:appendix_experiments}

\begin{figure}[t]
  \centering
  \includegraphics[height=9cm]{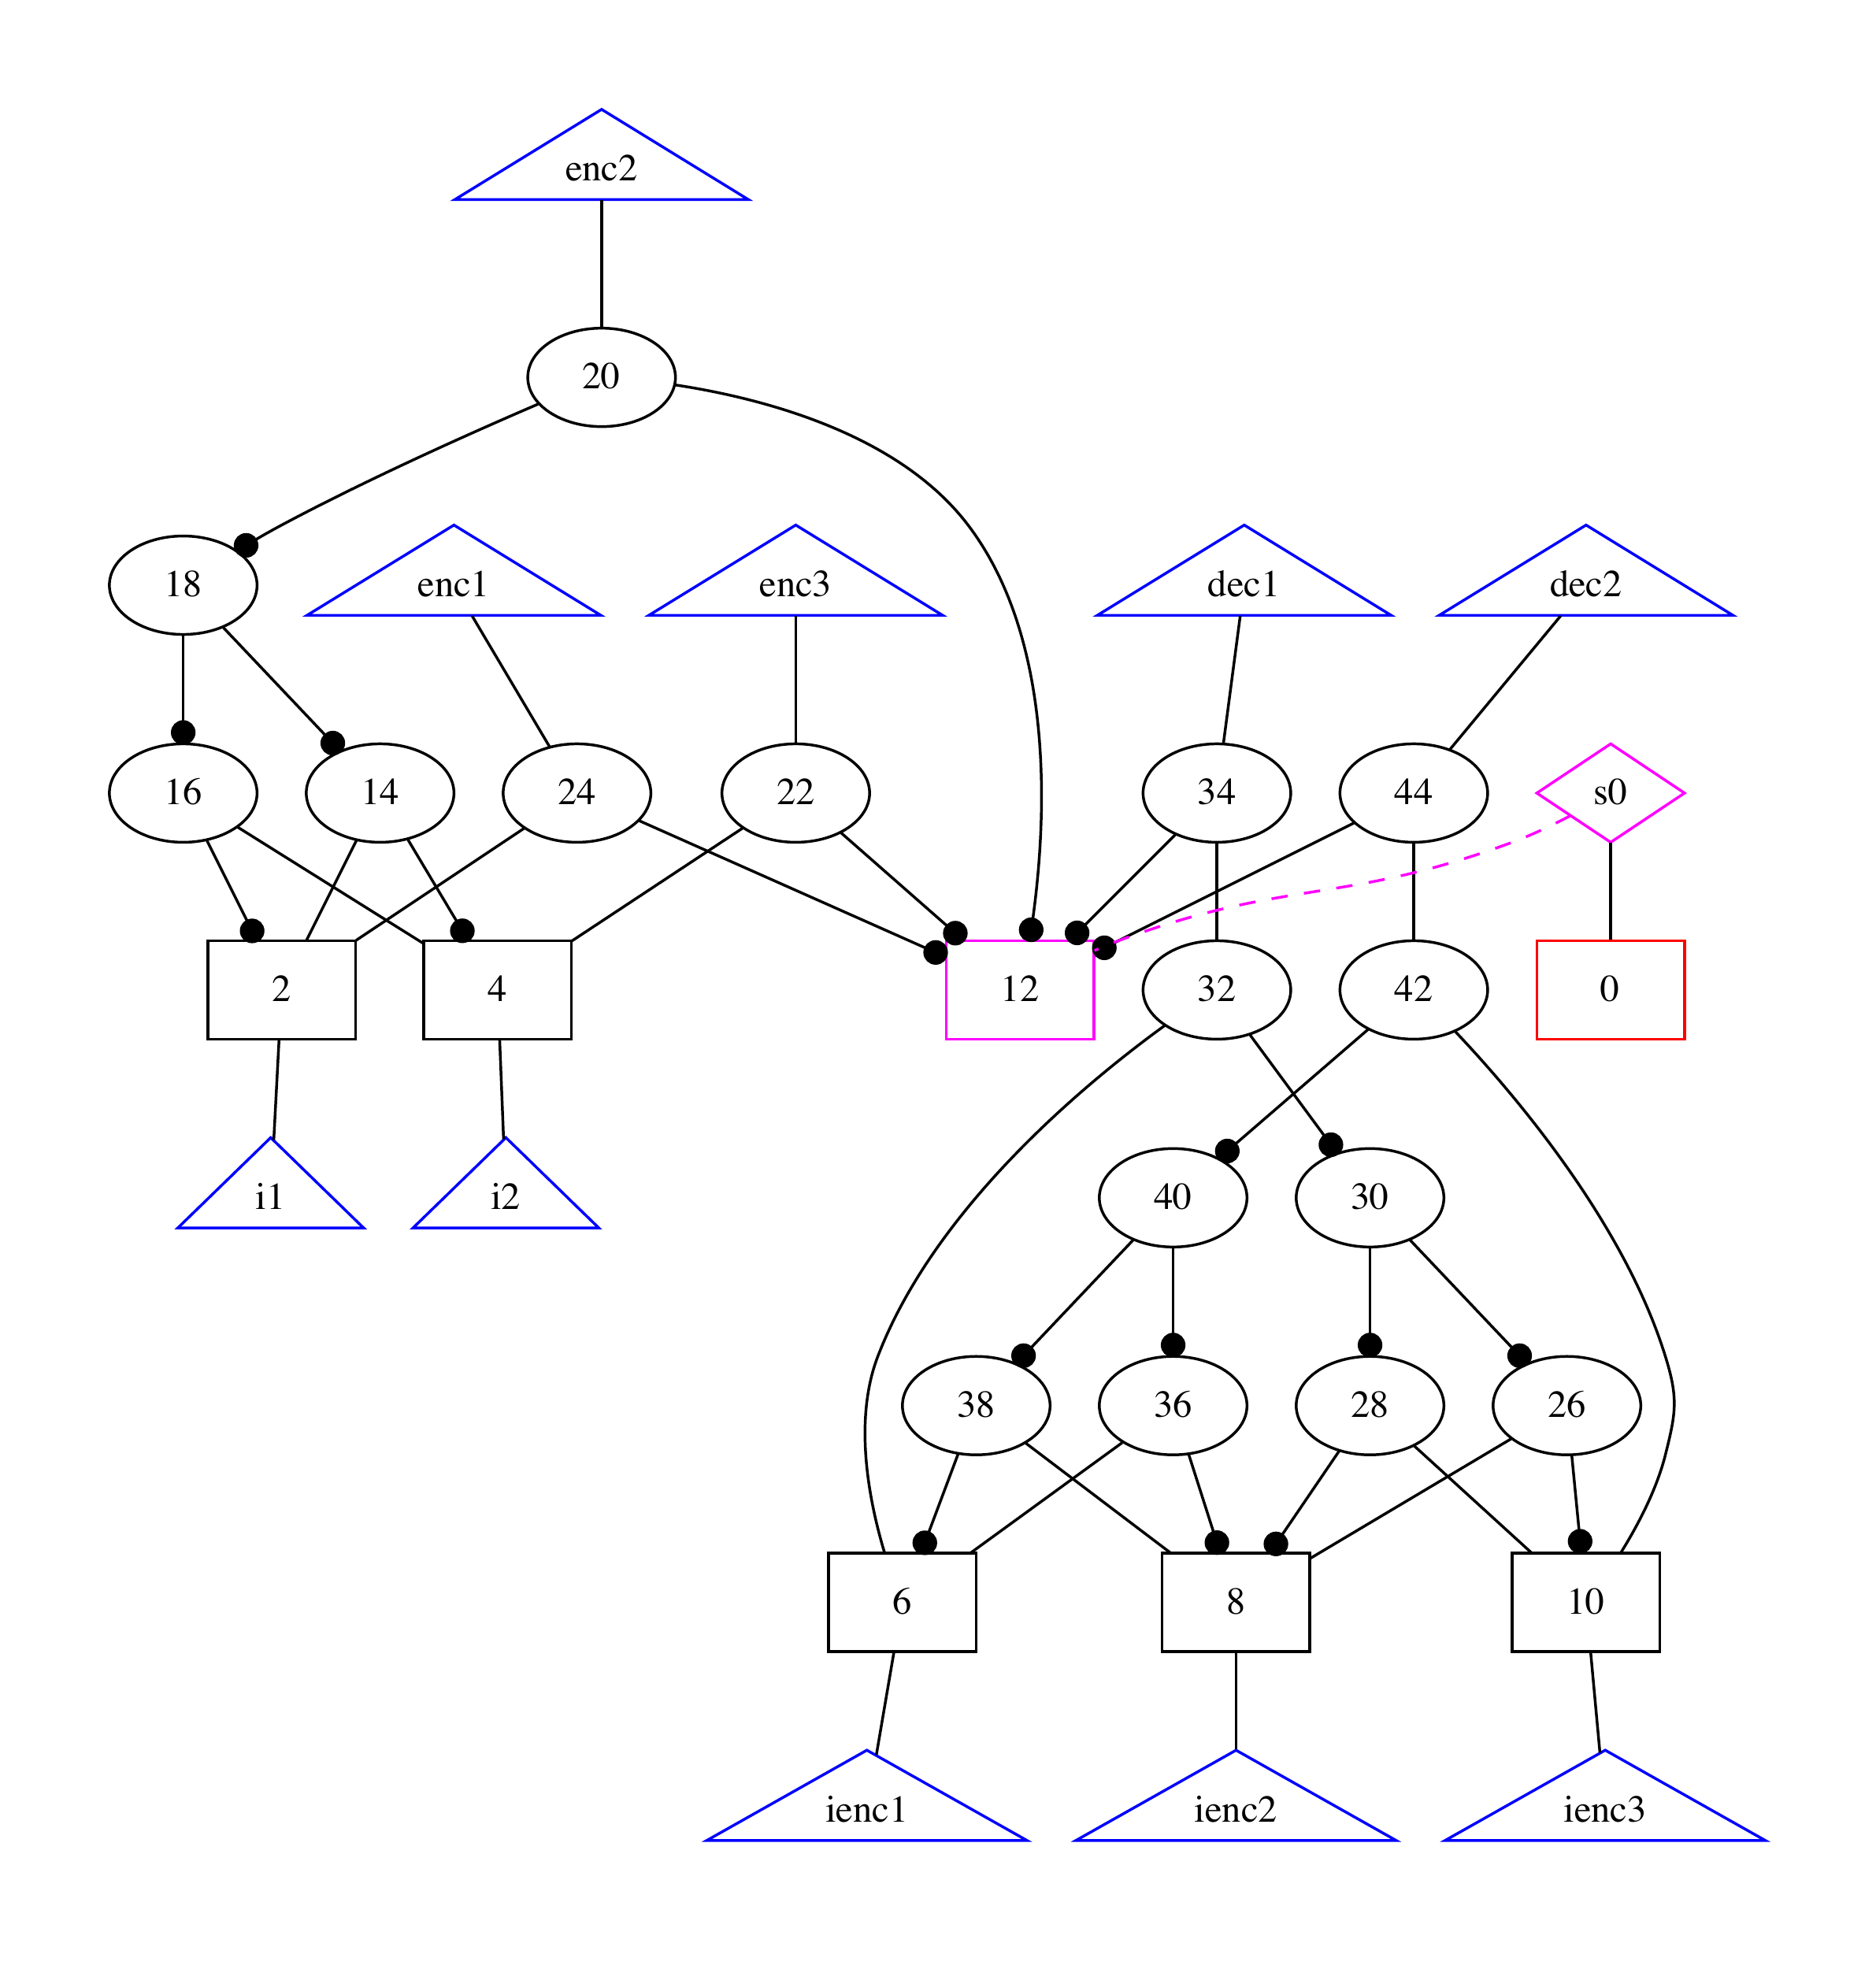}
  \caption{AIGER solution for encoder with 2 input bits and 3 encoded bits.}
  \label{fig:encoder-decider-2-3-solution}
\end{figure}

%-------------------------------------------------------------------------------
\paragraph{CAP Theorem.}
%-------------------------------------------------------------------------------

We recap the formal encoding~\cite{journals/corr/FinkbeinerT15} using $\hyperltl$.
There are two differences, we allow for acyclic architectures and we show the Mealy version (the Moore version needs $\X_3$ before the output).
We assume there is a fixed number $n$ of nodes, that every node implements the same service, and that there are direct communication links between all nodes.
We use the variables $\textit{req}_i$ and $\textit{out}_i$ to denote input and output of node $i$, respectively.
The consistency and availability requirements are encoded as the LTL formulas  $\G (\bigwedge_{1 \leq i < n} \textit{out}_i \leftrightarrow \textit{out}_{i+1})$ and $\G ((\bigvee_{1 \leq i \leq n} \textit{req}_i) \leftrightarrow (\bigvee_{1 \leq i \leq n} \textit{out}_i) )$.
The partition tolerance is modeled in a way that there is always at most one node partitioned from the rest of the system.
For two nodes, we get the $\ltl$ formula
\begin{equation*}
  \left( \G (\textit{chan}_1 \leftrightarrow \textit{com}_1) \lor \G (\textit{chan}_2 \leftrightarrow \textit{com}_2)  \right)
  \rightarrow
  \G ( (\textit{out}_1 \leftrightarrow \textit{out}_2) \land ( (\textit{req}_1 \lor \textit{req}_2) \leftrightarrow (\textit{out}_1 \lor \textit{out}_2 )) )
\end{equation*}
and additionally the $\hyperltl$ constraints $\dep{\set{\textit{req}_1,\textit{chan}_2}}{\set{\textit{com}_1,\textit{out}_1}}$ and $\dep{\set{\textit{req}_2,\textit{chan}_1}}{\set{\textit{com}_2,\textit{out}_2}}$.

%-------------------------------------------------------------------------------
\paragraph{Long-term information flow.}
%-------------------------------------------------------------------------------

We give the $\ltl$ specification used in the benchmarks in the following
\begin{align*}
    &\textit{idle} \\
    & \G ((\textit{idle} \land \neg\textit{send}) \rightarrow \X \textit{idle})\\
    &\G ((\textit{idle} \land \textit{send}) \rightarrow ((\X \textit{start}) \land (\X_2 \textit{transmit}) \land (\X_2 \textit{data} \leftrightarrow \textit{in}) ) )\\
    &\G (\textit{transmit} \rightarrow (\X \textit{waitForAck}))\\
    &\G ((\textit{waitForAck} \land \textit{ack}) \leftrightarrow (\X \textit{success}))\\
    &\G ((\textit{waitForAck} \land \neg\textit{ack}) \leftrightarrow (\X \textit{failure}))\\
    &\G (\textit{success} \rightarrow (\X \textit{idle}))\\
    &\G (\textit{failure} \rightarrow (\X \textit{idle}))\\
    &\G (\textit{mutex}(\textit{idle}, \textit{start}, \textit{transmit}, \textit{waitForAck}, \textit{success}, \textit{failure}))\\
\end{align*}
Additionally, we used the following $\hyperltl$ specifications
\begin{align*}
  &\forall \pi \forall \pi'\ldot (\G ( (\textit{send}_\pi \leftrightarrow \textit{send}_{\pi'}) \land (\textit{ack}_\pi \leftrightarrow \textit{ack}_{\pi'}) ) ) \rightarrow \G (\textit{data}_\pi \leftrightarrow \textit{data}_{\pi'}) \\
  &\forall \pi \forall \pi'\ldot (\G ( (\textit{send}_\pi \leftrightarrow \textit{send}_{\pi'}) \land (\textit{ack}_\pi \leftrightarrow \textit{ack}_{\pi'}) ) )\\
  &{}\rightarrow ( \G ( (\textit{send}_\pi \leftrightarrow \textit{send}_{\pi'}) \land (\textit{ack}_\pi \leftrightarrow \textit{ack}_{\pi'}) \land (\textit{in}_\pi \leftrightarrow \textit{in}_{\pi'}) ) \rightarrow \F\G (\textit{data}_\pi \leftrightarrow \textit{data}_{\pi'}) )
\end{align*}

\begin{figure}
  \input{tikz/dining_cryptographers}
  \caption{Architecture for the dining cryptographers}
  \label{fig:dining-cryptographers}  
\end{figure}
